# Supplementary material for: Co-Learning Empirical Games and World Models
Source: arXiv:2305.14223 source file (2023-05-23)
Supplement: Supplementary file 1 [file symbols.tex]

Bolt typeface refers to the joint across all players.
Subscript is used to denote a specific player $s_i$, or to denote all but a specific player $s_{-i}$.

\begin{center}
\begin{tabular}{ll}
    $h\in\mathcal{H}$ & World state \\ 
    $t\in\mathcal{T}$ & Time \\
    $o\in\mathcal{O}$ & Observation \\
    $a\in\mathcal{A}$ & Action \\
    $r\in\mathcal{R}$ & Reward \\
    $m^\pi\in\mathcal{M}^\pi$ & Agent's memory (recurrent state) \\
    $s\equiv(m^\pi, o)$ & Information State \\
    $\mathcal{S}\equiv(\mathcal{M}^\pi,\mathcal{O})$ & Information-State Space \\
    $(s^t, a^t, r^{t+1}, s^{t+1})$ & Transition or Experience \\
    $\tau$ & Sequence, or trajectory, of experiences. \\
    $\pi:\mathcal{O}\times\mathcal{M}^\pi\to\Delta(\mathcal{A})$ & Policy \\
    $\Pi$ & Policy Space \\
    $\sigma:\Pi\to\mathbb{R}$ & Strategy \\
    $\Sigma$ & Strategy Space \\
    $p:\mathcal{H}\times\mathbfcal{A}\to\Delta(\mathcal{H})\times\Delta(\mathbfcal{R})$ & Transition dynamics \\
    $U:\bm\Pi\to\mathbb{R}^n$ & Utility function \\ 
    $n$ & Number of players in a game \\
    $\Gamma\gets (\bm\Pi, U, n)$ & Normal-Form Game \\
    $\hat\Gamma\gets (\bm{\hat\Pi}, \hat{U}, n)$ & Empirical Normal-Form Game \\
    $\mathcal{B}$ & Replay Buffer \\
    $m^w\in\mathcal{M}^w$ & World model's memory (recurrent state) \\
    $w:\mathbfcal{O}\times\mathbfcal{A}\times\mathcal{M}^w\to\mathbfcal{O}\times\mathbfcal{R}$ & Agent world model
\end{tabular}
\end{center}
